# Supplementary material for: Testing the Number of Components in Finite Mixture Normal Regression Model with Panel Data
Source: arXiv:2210.02824 source file (2023-06-02)
Supplement: Supplementary file 1 [file FM_appendixa_DQM.tex]

%***************************************************************************
%       Quadratic expansion
%***************************************************************************
This appendix derives a Le Cam's differentiable in quadratic mean (DQM) type expansion, which is useful for proving Lemma 4.
\cite{Liu2003} derives a DQM under the loss of identifiability in terms of the generalized score function. \cite{Kasahara2019} develops a similar expansion
that accommodates mixtures of multivariate normal distributions.
Lemmas \ref{lemma:KS2018_lemma4} and \ref{lemma:KS2018_lemma5} follow Lemmas 4 and 5 of \cite{Kasahara2019} and \cite{Liu2003}.

Let $\bs{\vartheta}$ be a parameter vector, and let $g(\bs{w},\bs{\theta})$ denote the density of $\bs{w}$. Let $L_n(\bs{\vartheta}):= \sum_{i=1}^n \log g(\bs{W}_i,\bs{\vartheta}) $ denote the log-likelihood function. Split $\bs{\vartheta} = (\bs{\psi}^\top,\bs{\pi}^\top)^\top$ and write  $L_n(\bs{\vartheta}):=  L_n(\bs{\psi},\bs{\pi})$. $\pi$ is the part of $\bs{\vartheta}$ that is unidentified under the null hypothesis.
Denote the true parameter value of $\bs{\psi}$ by $\bs{\psi}^*$, and denote the set of $(\bs{\psi},\bs{\pi})$ corresponding to the null hypothesis by $\Gamma^* = \{ (\bs{\psi},\bs{\pi}) \in \Theta: \bs{\psi} = \bs{\psi}^*\}$.
Let $t(\bs{\vartheta})$ be a continuous function of $\bs{\vartheta}$ such that $t(\bs{\vartheta}) = 0$ if and only if $\bs{\psi} = \bs{\psi}^*$. For $\epsilon > 0$, define a neighborhood of $\Gamma^*$ by
\[ \mathcal{N}_{\epsilon} = \{ \bs{\vartheta} \in \Theta: |t(\bs{\vartheta})| < \epsilon \}. \]

We establish a general quadratic expansion that expresses $ L_n(\bs{\psi},\bs{\pi}) -  L_n(\bs{\psi}^*,\bs{\pi})$ as a quadratic function of $\bs{t(\bs{\vartheta})}$ for $\bs{\vartheta} \in \mathcal{N}_{\epsilon}$. Denote the density ratio by
\begin{equation}\label{eq:l_def}
l(\bs{w};\bs{\vartheta}): = \frac{g(\bs{w};\bs{\psi},\bs{\pi})}{g(\bs{w};\bs{\psi}^*,\bs{\pi})},
\end{equation}
so that $L_n(\bs{\psi},\bs{\pi}) - L_n(\bs{\psi}^*,\bs{\pi}) = \sum_{i=1}^n \log l(\bs{W}_i,\bs{\vartheta})$.
We assume that $l(\bs{w},\bs{\vartheta})$ can be expanded around $l(\bs{w},\bs{\vartheta}^*)=1$ as follows, where Assumption \ref{assumption_l_expansion} follows Assumption 6 in \cite{Kasahara2019}.

\begin{assumption}\label{assumption_l_expansion}
$l(\bs{w},\bs{\vartheta}) - 1$ admits an expansion
\begin{equation*}
    l(\bs{w},\bs{\vartheta}) - 1 = t(\bs{\vartheta})^\top s(\bs{w},\bs{\pi}) + r(\bs{w}, \bs{\vartheta}),
\end{equation*}
where $s(\bs{w},\pi) $ and $r(\bs{w},\vartheta)$ satisfy some $C \in (0,\infty)$ and $\epsilon > 0$.
(a) $ \mathrm{E} \sup_{\pi \in \Theta_{\pi}} |s(\bs{W}, \bs{\pi})| < C$, (b) $\sup_{\pi \in \Theta_{\pi}} |P_n(s(\bs{w},\bs{\pi})s(\bs{w},\pi)^\top ) - \bs{\mathcal{I}}_{\pi} | = o_p(1)$ with $ 0 < \inf_{\pi \in \Theta_{\pi}} \lambda_{min}(\mathcal{I}_{\pi}) < \sup_{\pi \in \Theta_{\pi}} \lambda_{max}(\mathcal{I}_{\pi}) < C$, 
(c) $E[\sup_{\vartheta \in \mathcal{N}_{\epsilon}}[r(\bs{W};\bs{\vartheta}) / (|t( \bs{\vartheta})| | \bs{\psi} - \bs{\psi}^*|)^2] < \infty$,
(d)  $\sup_{\bs{\vartheta} \in \mathcal{N}_{\epsilon} }  [r(\bs{W};\bs{\vartheta}) / (|t(\bs{\vartheta})| |\bs{\psi} - \bs{\psi}^*|)] = O_p(1) $, (e) $\sup_{\pi \in \Theta_{\pi}} |\nu_n(s(\bs{w};\bs{\pi})) | = O_p(1)$.
\end{assumption}

We first establish an expansion $L_n(\psi,\pi)$ in a neighborhood $\mathcal{N}_{c/\sqrt{n}}$ that holds for any $c > 0$.
\begin{lemma}\label{lemma:KS2018_lemma4}
    Suppose that Assumption \ref{assumption_l_expansion} (a)--(d) holds. Then, for all $c > 0$,
    $$ \sup_{\vartheta \in \mathcal{N}_{c / \sqrt{n}}} | L_n(\bs{\psi},\bs{\pi}) - L_n(\bs{\psi}^*,\bs{\pi}) - \sqrt{n} \bs{t}(\bs{\vartheta})^\top \nu_n(\bs{s}(\bs{w},\bs{\pi}))+ \bs{t}(\bs{\vartheta})^\top \bs{\mathcal{I}_{\pi}} \bs{t}(\bs{\vartheta})| = o_p(1).$$
\end{lemma}
\begin{proof}[Proof of Lemma \ref{lemma:KS2018_lemma4}]
    Define $h(\bs{w},\bs{\vartheta}) := \sqrt{l(\bs{w},\bs{\vartheta})} - 1 .$
    By applying the Taylor expansion of $2 \log(1 + x) = 2 x - x^2 (1 + o(1))$ for small $x$, we have, uniformly for $\bs{\vartheta} \in \mathcal{N}_{c/\sqrt{n}}$,
    \begin{equation}\label{eq:quadratic_expansion_mean}
    L_n(\bs{\psi},\bs{\pi}) - L_n(\bs{\psi}^*,\bs{\pi}) = 2 \sum_{i=1}^n \log( 1 + h(\bs{w}_i,\bs{\vartheta})) = n P_n( 2 h(\bs{w},\bs{\vartheta}) - [1 + o_p(1)] h(\bs{w},\bs{\vartheta})^2 ).
    \end{equation}

The stated result holds if we show

\begin{eqnarray}
         \sup_{\bs{\vartheta} \in \mathcal{N}_{c/\sqrt{n}}} | n P_n \Big( h(\bs{w}_i,\bs{\vartheta}))^2 \Big) - n \bs{t}(\bs{\vartheta})^\top \mathcal{I}_{\pi} \bs{t}(\bs{\vartheta}) /4 | = o_p(1)  \label{eq:KS_lemma_4_1}\\
         \sup_{\bs{\vartheta} \in \mathcal{N}_{c/\sqrt{n}}}  | n P_n \Big( h(\bs{w}_i,\bs{\vartheta})) \Big) - \sqrt{n} \bs{t}(\bs{\vartheta})^\top \nu_n (\bs{s}(\bs{w}))/2 + n \bs{t}(\bs{\vartheta})^\top \mathcal{I}_{\pi} \bs{t}(\bs{\vartheta}) /8 | = o_p(1) \label{eq:KS_lemma_4_2},
  \end{eqnarray}

    because the right-hand side of (\ref{eq:quadratic_expansion_mean}) equals $\sqrt{n} \bs{t}(\bs{\vartheta})^\top \nu_n(\bs{s}(\bs{w})) - n \bs{t}(\bs{\vartheta})^\top \bs{\mathcal{I}}_{\bs{\pi}} \bs{t}(\bs{\vartheta})/2$ uniformly in $\bs{\vartheta} \in \mathcal{N}_{c / \sqrt{n}}$.

    To show equation (\ref{eq:KS_lemma_4_1}), write \[4 P_n \Big( h(\bs{w}_i,\bs{\vartheta}))^2 \Big) = P_n \Bigg( \frac{4 (l(\bs{w},\vartheta) -1 )^2}{ (\sqrt{l(\bs{w},\vartheta)} + 1 )^2} \Bigg) = P_n(l(\bs{w},\vartheta) - 1)^2 - P_n\Bigg((l(\bs{w},\vartheta)-1)^3\frac{\sqrt{l(\bs{w},\vartheta)}+3}{ (\sqrt{l(\bs{w},\vartheta)}+1)^3 }\Bigg).\]
    If follows from Assumption \ref{assumption_l_expansion}(a)--(c) and $(\E(XY))^2 \le \E|X|^2 \E|Y|^2$ that, uniformly for $\bs{\vartheta} \in \mathcal{N}_{\epsilon}$,
    \begin{equation}\label{eq:P_l_convergence}
        \begin{split}
        P_n(l(\bs{w},\vartheta) - 1)^2 & = \bs{t}(\bs{\vartheta})^\top P_n \big(\bs{s}(\bs{w})\bs{s}(\bs{w},\bs{\vartheta})^\top\big)  \bs{t}(\bs{\vartheta}) + 2 \bs{t}(\bs{\vartheta})^\top P_n\big(\bs{s}(\bs{w},\bs{\vartheta}) \bs{r}(\bs{w},\bs{\vartheta})\big) + P_n(\bs{r}(\bs{w}))^2 \\
        & = (1 + o_p(1)) \bs{t}(\bs{\vartheta})^\top \bs{\mathcal{I}}_{\bs{\pi}} \bs{t}(\bs{\vartheta}) + O_p(|\bs{t}(\bs{\vartheta})|^2 | \bs{\psi} - \bs{\psi}^* |).
        \end{split}
    \end{equation}
    Therefore, we have $P_n(l(\bs{w},\vartheta) - 1)^2  = \bs{t}(\bs{\vartheta})^\top \bs{\mathcal{I}}_{\bs{\pi}} \bs{t}(\bs{\vartheta}) + o_p(n^{-1})$.
    Note that if the data $W_1,\ldots,W_n$ are random variables with $\max_{1\le i \le n} \E| W_i|^q < C$ for some $q > 0$ and $C < \infty$, then we have $\max_{1 \le i \le n} |W_i| = o_p(n^{1/q})$.
    Therefore, from Assumption \ref{assumption_l_expansion}(a) and (c), we have
    \begin{equation}
    \max_{1 \le i \le n} \sup_{\bs{\vartheta} \in \mathcal{N}_{c/\sqrt{n}}} | l(\bs{W}_i,\bs{\vartheta}) -1 | = \max_{1 \le i \le n} \sup_{\bs{\vartheta} \in \mathcal{N}_{c/\sqrt{n}}} | \bs{t}(\bs{\vartheta})^\top \bs{s}(\bs{W}_i,\bs{\pi}) + r(\bs{W}_i,\bs{\vartheta}) | = o_p(1).
    \end{equation}
   Therefore, $P_n\Bigg((l(\bs{w},\vartheta)-1)^3\frac{\sqrt{l(\bs{w},\vartheta)}+3}{ (\sqrt{l(\bs{w},\vartheta)}+1)^3 }\Bigg) = o_p(n^{-1})$, and (\ref{eq:KS_lemma_4_1}) follows.

   We proceed to show (\ref{eq:KS_lemma_4_2}). Consider the following expansion of $h(\bs{w},\bs{\vartheta})$:
   \begin{equation}\label{eq:KS_lemma_4_2_exp}
   	h(\bs{w},\bs{\vartheta}) = (l(\bs{w},\bs{\vartheta}) - 1) / 2 - h(\bs{w},\bs{\vartheta})^2 /2 = (\bs{t}(\bs{\vartheta})^\top) s(\bs{w},\bs{\pi}) + r(\bs{w},\bs{\vartheta})/2 - h(\bs{w},\bs{\vartheta})^2 / 2.
   \end{equation}
   Then, (\ref{eq:KS_lemma_4_2}) follows from (\ref{eq:KS_lemma_4_1}), (\ref{eq:KS_lemma_4_2_exp}), Assumption \ref{assumption_l_expansion}(d), and the stated result follows.
\end{proof}

Lemma \ref{lemma:KS2018_lemma5} expands $L_n(\bs{\psi},\bs{\pi})$ in $A_{n \epsilon} := \{ \bs{\vartheta} \in \mathcal{N}_{\epsilon} : L_n(\bs{\psi},\bs{\pi}) - L_n(\bs{\psi}^*,\bs{\pi}) \} \ge - \delta$  for  $\delta \in (0,\infty)$.
This lemma is useful for deriving the asymptotic distribution of the LRTS because a consistent MLE is in $A_{n\epsilon}(\delta)$ by definition.
Define $O_{p \epsilon}(\cdot)$ and $o_{p \epsilon}(\cdot)$ as in Appendix \ref{sec:appendixb}.

\begin{lemma}\label{lemma:KS2018_lemma5}
Suppose that Assumption \ref{assumption_l_expansion} holds. Then, for any $\delta > 0$, (a) $\sup_{\vartheta in A_{n \epsilon}(\delta)} | \bs{t}(\bs{\vartheta}) | = O_{p \epsilon}(n^{-1/2})$ and (b) $\sup_{\bs{\vartheta} \in A_{n \epsilon}(\delta} | L_n(\bs{\psi},\bs{\pi}) - L_n(\bs{\psi}^*,\bs{\pi}) - \sqrt{n} \bs{t}(\bs{\vartheta})^\top \nu_n(\bs{s}(\bs{w},\bs{\pi})) + n \bs{t}(\bs{\vartheta})^\top \bs{\mathcal{I}}_{\bs{\pi}} \bs{t}(\bs{\vartheta}) / 2 | = o_{p\epsilon}(1). $
\end{lemma}
\begin{proof}[Proof of Lemma \ref{lemma:KS2018_lemma5}]
For part (a), applying the inequality $\log(1+x) \le x$ to the log-likelihood ratio function and with (\ref{eq:KS_lemma_4_2_exp}) gives
\begin{equation}\label{eq:logL_expansion_h}
L_n(\bs{\psi},\bs{\pi}) - L_n(\bs{\psi}^*,\bs{\pi}) = 2 \sum_{i=1}^n \log(1 + h(\bs{W}_i,\bs{\vartheta})) \le 2 n  P_n (h(\bs{w},\bs{\vartheta})) = \sqrt{n} \nu_n(l(\bs{w},\bs{\vartheta})) - nP_n (h(\bs{w},\bs{\vartheta})^2).
\end{equation}
We derive a lower bound on $P_n (h(\bs{w},\bs{\vartheta})^2)$. Observe that $h(\bs{w},\bs{\vartheta})^2 = (l(\bs{w},\bs{\vartheta}))^2 / (\sqrt{l(\bs{w},\bs{\vartheta}) } + 1)^2 \ge \ind \{ l(\bs{w},\bs{\vartheta}) \le \kappa \} (l(\bs{w},\bs{\vartheta}) - 1)^2 / ( \sqrt{\kappa} + 1 )^2 $ for any $\kappa > 1$.
Therefore, \begin{equation*}
\begin{split}
P_n(h(\bs{w},\bs{\vartheta})^2) & \ge (\sqrt{\kappa} + 1)^{-2} P_n \left(\ind \{l(\bs{w},\bs{\vartheta}) \le \kappa\} (l(\bs{w},\bs{\vartheta} )-1 )^2 \right) \\
& \ge (\sqrt{\kappa} + 1)^{-2} \Big[  P_n  (l(\bs{w},\bs{\vartheta}) -1 )^2 )) -  P_n \left(\ind \{l(\bs{w},\bs{\vartheta}) > \kappa\} (l(\bs{w},\bs{\vartheta} )-1 )^2 \right) \Big].
\end{split}
\end{equation*}
Let $B : = \sup_{\bs{\vartheta} \in \mathcal{N}_{\epsilon}}|l(\bs{w},\bs{\vartheta}) - 1|$. From Assumption \ref{assumption_l_expansion}(a) and (c), we have $\E B^2 < \infty$, and hence $\lim_{\kappa \to \infty} \sup_{\vartheta \in \mathcal{N}_{\epsilon}} P_n( \ind\{l(\bs{w},\bs{\vartheta}) > \kappa\}(l(\bs{w},\bs{\vartheta})-1)^2) \le \lim_{\kappa \to \infty} P_n( \ind \{ B + 1 > \kappa \} B^2 )$  almost surely. Let $\tau = (\sqrt{\kappa} + 1)^{-2} / 2$. With a sufficiently large $\kappa$, it follows from (\ref{eq:P_l_convergence}), uniformly for $\bs{\vartheta} \in \mathcal{N}_{\epsilon}$, that
\begin{equation}\label{eq:KS_lemma_5_2}
P_n(h(\bs{w},\bs{\vartheta})^2) \ge \tau ( 1+ o_p(1)) \big(\bs{t}(\bs{\vartheta})^\top \bs{\mathcal{I}}_{\bs{\pi}}\bs{t}( \bs{\vartheta}) \big) + O_p(|\bs{t}(\bs{\vartheta})|^2 |\bs{\psi} - \bs{\psi}^*|  ).
\end{equation}

Because $\sqrt{n}\nu_n(l(\bs{w},\bs{\vartheta})-1) = \sqrt{n} \bs{t}(\bs{\vartheta})^\top [ \nu_n(\bs{s}(\bs{w},\bs{\pi})) +O_p(1) ]$ from Assumption \ref{assumption_l_expansion}(d), it follows from (\ref{eq:logL_expansion_h}) and (\ref{eq:KS_lemma_5_2}) that
\begin{equation}\label{eq:KS_lemma_5_3}
\begin{split}
    - \delta & \le L_n(\psi,\pi) - L_n(\psi^*,\pi) \\
    & \le \sqrt{n} \bs{t}(\bs{\vartheta})\t [\nu_n (s(\bs{w}, \bs{\pi})) + O_p(1)]  - \tau (1 + o_p(1)) n \bs{t}(\bs{\vartheta})\t \mathcal{I}_{\pi} \bs{t}(\bs{\vartheta}) + O_p(n |\bs{t}(\bs{\vartheta})|^2 |\bs{\psi} - \bs{\psi}^*|).
\end{split}\end{equation}
\noindent Let $\bs{T}_n = \mathcal{I}_{\pi}^{1/2} \sqrt{n} \bs{t}(\bs{\vartheta})$. From (\ref{eq:KS_lemma_5_3}), Assumption \ref{assumption_l_expansion}(c) and (e), and the fact that $\bs{\psi} - \bs{\psi}^* \to 0$ if $\bs{t}(\bs{\vartheta}) \to 0$, we obtain the following results: for any $\Delta > 0$, there exist $\epsilon > 0$ and $M,n_0 < \infty$ such that
\begin{equation}
\text{Pr} \Bigg( \inf_{\vartheta \in \mathcal{N}_{\epsilon}} ( |\bs{T}_n | M - (\tau/2)|\bs{T}_n|^2 + M) \ge 0 \Bigg) \ge 1 - \Delta, \text{ for all } n > n_0.
\end{equation}
Rearranging the terms inside $\text{Pr}(\cdot)$ gives $\sup_{\bs{\vartheta} \in \mathcal{N}_{\epsilon}} (|\bs{T}_n| -( M /\tau))^2 \le 2 M / \tau + (M / \tau)^2$, and part (a) follows. Part (b) follows part (a) and Lemma \ref{lemma:KS2018_lemma4}.
%\ref{eq:logL_expansion_h}
\end{proof}
