# Supplementary material for: Testing the Number of Components in Finite Mixture Normal Regression Model with Panel Data
Source: arXiv:2210.02824 source file (2023-06-02)
Supplement: Supplementary file 2 [file FM_appendixa_DQM_logL.tex]

This appendix derives a Le Cam's differentiable in quadratic mean (DQM) type of expansion that is useful for proving Lemma \ref{lemma:KS2018_lemma1} under the finite mixture model of normal panel regression.
\cite{Liu2003} develop a DQM expansion under the loss of identifiability in terms of a generalized score function.
Lemma \ref{lemma:KS2018_lemma1} follow  Lemmas 1-3 of \cite{Kasahara2019}.
Lemma \ref{lemma:KS2018_lemma1} considers the case of testing $H_0: M = 1$ against $H_A: M = 2$.
For a sequence $X_{n \epsilon}$ indexed by $n = 1,\ldots, $ and $\epsilon$, we write $X_{n \epsilon} = O_{p \epsilon}(a_n)$ if for any $\Delta > 0$, there exist $\epsilon >  0$ and $M, n_0 < \infty$ such that $\mathbbm{P}(|X_{n \epsilon} / a_n | \le M) \ge 1 - \Delta $ for all $n > n_0$.
We write $X_{n \epsilon} = o_{p \epsilon}(a_n)$ if for any $\Delta_1, \Delta_2 > 0$, there exist $\epsilon > 0$ and $n_0$ such that $\mathbbm{P}(|X_{n \epsilon}/ a_n| \le \Delta_1) \ge \Delta_2$ for all $n > n_0$.
Loosely, $X_{n \epsilon} = O_{p \epsilon}(a_n)$ and $X_{n \epsilon} = o_{p \epsilon}(a_n)$ mean that $X_{n \epsilon} = O_p(a_n)$ and $X_{n \epsilon} = o_p(a_n)$, respectively, when $\epsilon$ is sufficiently small.

\begin{lemma}\label{lemma:KS2018_lemma1}
Suppose that Assumptions \ref{assumption:1} and \ref{assumption:2} hold and $\bs{w} = (y,\bs{x}^\top,\bs{z}^\top)^\top$ has the density of $f(\bs{w};\bs{\gamma},\bs{\theta})$ defined in (\ref{eq:f1}).
Let $L_n(\psi,\alpha) = \sum_{i=1}^n \log g(\bs{W}_i;\bs{\psi},\alpha)$ with $g(\bs{w};\bs{\psi},\alpha)$ defined in equation (\ref{eq:repar}). For $\alpha \in(0,1)$, define $s(\bs{w})$ and $t(\bs{\psi},\alpha)$
as the score function and the collection of parameters defined in (\ref{eq:s_1}) and (\ref{eq:t_1}).
In addition, let $\mathcal{N}_{\epsilon} = \{ \vartheta_2 \in \Theta_{\vartheta_2} : |t(\psi,\alpha)| < \epsilon  \}$ and $\bs{\mathcal{I}} = E [s(\bs{w})s(\bs{w})^\top]$. Then, for $\epsilon_{\sigma} \in (0,1)$ and any $\delta > 0$,
we have
\begin{enumerate}[label=(\alph*)]
    \item $\sup_{\vartheta_2 \in A_{n\epsilon}} |t(\bs{\psi},\alpha)| = O_{p \epsilon}(n^{-\frac{1}{2}})$;
    \item $ \sup_{\vartheta_2 \in A_{n\epsilon}(\delta)} \left| L_n(\bs{\psi},\alpha) - L_n(\bs{\psi}^*,\alpha) - \sqrt{n} t(\bs{\psi},\alpha)^\top \nu_n(s(x,z)) + n t(\bs{\psi},\alpha)^\top \bs{\mathcal{I}} t(\bs{\psi},\alpha)/2 \right| = o_{p \epsilon}(1),$
    where $A_{n\epsilon}(\delta) = \{ \varepsilon_2 \in \mathcal{N}_{\epsilon} : L_n(\bs{\psi},\alpha) - L_n(\bs{\psi}^*,\alpha)  \ge -\delta \}$.
\end{enumerate}

\end{lemma}

\begin{proof}[Proof of Lemma \ref{lemma:KS2018_lemma1}]
First, we show  that $l(\bs{w},\bs{\psi},\alpha) = g(\bs{w},\bs{\psi},\alpha) / g(\bs{w},\bs{\psi}^*,\alpha)$ with $\bs{w} = (y,\bs{x}^\top,\bs{z}^\top)^\top$.
In this expansion, $l(\bs{w},\bs{\psi},\alpha)$ plays the role of $l(\bs{w},\bs{\vartheta})$ and $\bs{t}(\bs{w},\alpha)$ plays the role of $\bs{t}(\vartheta)$.
Observe that $\bs{t}(\bs{\psi},\alpha)$ defined in equation (\ref{eq:t_1}) satisfies $\bs{t}(\bs{\psi},\alpha) = 0$ if and only if $\psi = \psi^*$ because $\bs{\lambda} = 0$ if and only if $\theta_1 = \theta_2$. We expand $l(\bs{w};\bs{\psi},\alpha) - 1$ five times with respect to $\bs{\psi}$ and show that the expansion satisfies Assumption \ref{assumption_l_expansion}.

Define
\begin{equation}\label{eq:nu_psi_two_times}
    \nu(\bs{w},\vartheta_2) = (\nabla_{\psi} g(\bs{w},\bs{\psi},\alpha)^\top,\nabla_{\psi^{\otimes 2}} g(\bs{w},\bs{\psi},\alpha)^\top, \nabla_{\psi^{\otimes 3}} g(\bs{w},\bs{\psi},\alpha)^\top)\top /  g(\bs{w},\bs{\psi}^*,\alpha).
\end{equation}
Note that equation (\ref{eq:nu_psi_two_times}) satisfies $\E(\nu(\bs{w},\vartheta_2)) = 0$.
To apply Lemma \ref{lemma:KS2018_lemma5} to $l(\bs{w},\bs{\psi},\bs{\alpha})$, we first show
\begin{eqnarray}
\sup_{\bs{\vartheta} \in \mathcal{N}_{\epsilon}} | P_n[\bs{\nu}(\bs{w},\bs{\vartheta}_2) \bs{\nu}(\bs{w},\bs{\vartheta}_2)]^\top - \E[\bs{\nu}(\bs{W},\bs{\vartheta}_2) \bs{\nu}(\bs{W},\bs{\vartheta}_2)]^\top  | = o_p(1) \label{eq:lemma1_cond1}\\
\bs{\nu}(\bs{w},\bs{\vartheta}_2) \Rightarrow \bs{W}(\bs{\vartheta_{2}}), \label{eq:lemma1_cond2}
\end{eqnarray}
$\bs{W}(\bs{\vartheta_{2}})$ is a mean-zero continuous Gaussian process with $\E[\bs{W}(\bs{\vartheta_{2}}) \bs{W}(\bs{\vartheta_{2}})^\top] = \E [\bs{\nu}(\bs{w},\bs{\vartheta}_2) \bs{\nu}(\bs{w},\bs{\vartheta}_2)^\top ]$.
Equation (\ref{eq:lemma1_cond1}) holds because $[\bs{\nu}(\bs{w},\bs{\vartheta}_2) \bs{\nu}(\bs{w},\bs{\vartheta}_2)^\top ]$ satisfies a uniform law of large numbers (see Lemma 2.4 of \cite{Newey1994}) because $\bs{\vartheta}(\bs{w},\bs{\vartheta_{2}})$ is continuous in $\bs{\vartheta_{2}}$ and $\E \sup_{\bs{\vartheta_2} \in \mathcal{N}_{\epsilon}}[\bs{\vartheta}(\bs{w},\bs{\vartheta_{2}}) \bs{\vartheta}(\bs{w},\bs{\vartheta_{2}})^\top] < \infty$ from the property of the normal density and Assumption \ref{assumption:2}.
Equation (\ref{eq:lemma1_cond2}) follows from Theorem 10.2 of \cite{Pollard1990} if (i) $\bs{\Theta}_{\bs{\vartheta}_2}$ is totally bounded, (ii) the finite dimensional distribution of $\nu_n(\bs{w},\bs{\vartheta}_2)$ converges to the distribution of $\bs{W}(\bs{\vartheta_{2}})$, and (iii) $\{ \nu_n( \bs{w},\bs{\vartheta_{2}})]) : n \ge 1 \}$ is stochastically equicontinuous.
Condition (i) holds because $\bs{\Theta}_{\vartheta_{2}}$ is compact in the Euclidean space. Condition (ii) follows from Assumption \ref{assumption:2} and the multivariate CLT. Condition (iii) follows from Theorem 2 of \cite{Andrews1994} because $v(\bs{w},\bs{\vartheta}_2)$ is Lipschitz continuous in $\bs{\vartheta}_{2}$.

Note that the $(p+1)$-th order Taylor expansion of $g(\bs{\psi})$ around $\bs{\psi} = \bs{\psi}^*$ is given by $$ g(\bs{\psi}) = g(\bs{\psi^*}) + \sum_{j=1}^p \frac{1}{j!} \nabla_{(\bs{\psi}^{\otimes j})^\top}  g(\bs{\psi^*}) (\bs{\psi} - \bs{\psi}^*)^{\otimes j } + \frac{1}{(p+1)!}  \nabla_{(\bs{\psi}^{\otimes {p+1}})^\top} g(\bar{\bs{\psi}}) (\bs{\psi} - \bs{\psi}^*)^{\otimes ( p+1)},  $$
where $\bar{\bs{\psi}}$ lies between $\bs{\psi}$ and $\bs{\psi}^*$ and $\bar{\bs{\psi}}$  may differ from element to element of $\nabla_{(\bs{\psi}^{\otimes (p+1)})^\top} g(\bar{\bs{\psi}})$.

Let $g^*$ and $\nabla g^*$ denote $g(\bs{w};\bs{\psi},\alpha)$ and $\nabla g(\bs{w};\bs{\psi},\alpha)$, and let $\nabla \bar{g}$ denote $\nabla g(\bs{w};\bs{\psi},\alpha)$. Let $\dot{\bs{\psi}} := \bs{\psi} - \bs{\psi}^*$ and $\dot{\bs{\eta}} := \bs{\eta} - \bs{\eta}^*$. Expanding $l(\bs{w};\bs{\psi},\alpha)$ around $\bs{\psi}^*$ while fixing $\alpha$ and using Lemma \ref{lemma:KS2018_lemma7}, we can write $l(\bs{w};\bs{\psi},\alpha) - 1$ as
$$ l(\bs{w};\bs{\psi},\alpha) - 1 =  \bs{s}(\bs{w};\bs{\eta},\bs{\lambda}) + r(\bs{w};\bs{\eta},\bs{\lambda}) ,$$
where $$ \bs{s}(\bs{w};\bs{\eta},\bs{\lambda}) : \frac{\nabla_{\eta^\top} g^* }{g^*} \dot{\bs{\eta}} + \frac{1}{2!}\frac{\nabla_{(\bs{\lambda}^{\otimes 2})^\top} g^* }{g^*}  \bs{\lambda}^{\otimes 2}, $$
and
\begin{equation}\label{eq:r_expansion}
\begin{split}
r(\bs{w};\bs{\eta},\bs{\lambda}) = \frac{1}{2!} \frac{\nabla_{\bs{\eta}^{\otimes 2}}g^*}{g^*} \bs{\dot{\eta}}^{\otimes 2} + \frac{1}{3!} \frac{\nabla_{ (\eta^{\otimes 3})\t }g^*}{g^*} (\eta^{\otimes 3}) + \frac{3}{3!} \frac{\nabla_{ (\eta \otimes \bs{\lambda}^{\otimes 2})\t }g^*}{g^*} (\eta \otimes \bs{\lambda}^{\otimes 2}) + \frac{1}{3!} \frac{\nabla_{ (\lambda^{\otimes 3})\t }g^*}{g^*} (\lambda^{\otimes 3}),
\end{split}
\end{equation}
where $s(\bs{w};\bs{\eta},\bs{\lambda})$ is the leading term in the expansion. We first show $s(\bs{w};\bs{\eta},\bs{\lambda}) = \bs{t}(\bs{\psi},\alpha) \bs{s}(\bs{w})$
score and $\bs{t}(\bs{\psi},\alpha)$ defined in (\ref{eq:s_1}) and (\ref{eq:t_1}).
Let $f^*$ and $\nabla f^*$ denote $f(\bs{w};\bs{\gamma}^*,\bs{\theta}^*)$ and $\nabla f(\bs{w};\bs{\gamma}^*,\bs{\theta}^*)$.
The first term of $s(\bs{w};\bs{\eta},\bs{\lambda})$ is $(\nabla_{(\eta)^\top} g^* / g^* ) \dot{\bs{\eta}} = ( \nabla_{(\bs{\gamma}^\top,\bs{\theta}^\top)^\top } f^* / f) \bs{\dot{\eta}} $.
Using the result from Lemma \ref{lemma:KS2018_lemma7}, the second term of $s(\bs{w};\bs{\eta},\bs{\lambda})$ can be written as $\frac{1}{2!} \alpha(1-\alpha) ( \nabla_{\bs{\theta}^{\otimes 2}} f^* / f^*) \bs{\lambda}^{\otimes 2} $, and hence $s(\bs{w};\bs{\eta},\bs{\lambda}) = \bs{t}(\bs{\psi},\alpha)^\top \bs{s}(\bs{w})$.

From (\ref{eq:lemma1_cond1}) and (\ref{eq:lemma1_cond2}) and the property of normal density, $\bs{s}(\bs{w})$ satisfies Assumption \ref{assumption_l_expansion} (a), (b), and (e). We need to show that $r(\bs{w};\bs{\eta},\bs{\lambda})$ satisfies Assumption \ref{assumption_l_expansion} (c) and (d).
Following the proof of Lemma 1 in\cite{Kasahara2019}, we can show that $r(\bs{w};\bs{\eta},\bs{\lambda})$ can be expressed as $\bs{\xi} (\bs{w};\bs{\vartheta}) O(| \bs{\psi} - \bs{\psi}^*| |\bs{t}(\bs{\psi},\alpha)| )$, where $\sup_{\bs{\vartheta} \in \mathcal{N}_{\epsilon}} | \bs{\xi}(\bs{w};\bs{\vartheta})| \le  \sup_{\bs{\vartheta} \in \mathcal{N}_{\epsilon}} | \bs{\nu}(\bs{w};\bs{\vartheta})| $,
where $\bs{\nu}(\bs{w};\bs{\vartheta})$ is defined in (\ref{eq:nu_psi_two_times}). Then, Assumption \ref{assumption_l_expansion} follows from the property of the normal density and (\ref{eq:lemma1_cond2}).

First, write the first term on the right-hand side of (\ref{eq:r_expansion}) as $\frac{\nabla_{\bs{\eta}^{\otimes 2}}g^*}{g^*} O(|\bs{\dot{\eta}}|^2)$.
Second, write the second and third terms of (\ref{eq:r_expansion}) as $\frac{\nabla_{ (\psi^{\otimes 3})\t }g^*}{g^*} O(|\bs{\dot{\eta}}|) O(|\bs{\lambda}|)$.
Then, write the last term of (\ref{eq:r_expansion})  as $\frac{\nabla_{ (\psi^{\otimes 3})\t }g^*}{g^*} O(|\bs{\lambda}|^{\otimes 3})$.
Thus, the terms of (\ref{eq:r_expansion}) are $ \nu(\bs{w},\vartheta_2)O(|\psi - \psi^*||t(\psi,\alpha)|)$, and the stated result follows. 

\end{proof}
