# Supplementary material for: Testing the Number of Components in Finite Mixture Normal Regression Model with Panel Data
Source: arXiv:2210.02824 source file (2023-06-02)
Supplement: Supplementary file 3 [file FM_appendixc.tex]

\subsection{Score function}

Define the score functions $s_{\eta i} $ to be the score functions relevant to $\eta$, and define $s_{\lambda i}$ the score functions relevant $\lambda$. The reparameterized score functions are $s_i = (s_{\eta i}^\top,s_{\lambda i}^\top)^\top$, where
$s_{\eta i} : =
(s_{\mu i} ,s_{\beta i}^\top,s_{\sigma i},s_{\bs{\gamma} i}^\top)^\top$, $s_{\lambda i} = (s_{\lambda_{\mu \sigma} i},s_{\lambda_{\beta} i})$.  The score functions are as described in \ref{sec:appendixb}, where $H^b(\cdot)$ is defined as the $b$-th order Hermite polynomial. $H^1(t) = t$, $H^2(t) = t^2 - 1$ , $H^3(t) = t^3 - 3t$, and $H^4(t) = t^4 - 6t^2 + 3$.  Use $H^{b*}_{i,t}$ as short form of $\frac{1}{b!} \frac{1}{\sigma^* } H^{b}(\frac{y_{it} - \mu^* - x_{it}^\top \beta^* - z_{it}^\top \bs{\gamma}^* }{\sigma^*}) .$

\begin{equation}\label{score_1}
\begin{split}
s_{\eta i} = \begin{pmatrix}
	\sum_{t=1}^T  H^{1*}_{i,t} \\
	\sum_{t=1}^T  H^{1*}_{i,t}x_{it}\\
	\sum_{t=1}^T  H^{2*}_{i,t} \\
	\sum_{t=1}^T  H^{1*}_{i,t}z_{it}\\
	\end{pmatrix},s_{\lambda_{\mu \sigma} i} =
	\begin{pmatrix}
	\sum_{t=1}^T H^{2*}_{i,t} +  \frac{1}{2} \sum_{t=1}^T \sum_{s \neq t} H^{1*}_{1,i,t} H^{1*}_{i,s} \\
	3 \sum_{t=1}^T H^{4*}_{i,t} + \frac{1}{2} \sum_{t=1}^T \sum_{s \neq t} H^{2*}_{i,t} H^{2*}_{i,t}  \\
	3 \sum_{t=1}^T H^{3*}_{i,t} +  \sum_{t=1}^T \sum_{s \neq t} H^{1*}_{i,t} H^{2*}_{i,s} \\
	2 \sum_{t=1}^T H^{2*}_{i,t}x_{it} +  \sum_{t=1}^T \sum_{s \neq t} H^{1*}_{i,t}x_{it} H^{1*}_{i,s} \\
	3  \sum_{t=1}^T H^{3*}_{i,t}x_{it} + 2 \sum_{t=1}^T\sum_{s \neq t} H^{1*}_{i,t}x_{it} H^{2*}_{i,s}
	\end{pmatrix} , \\
	s_{\lambda_{\beta}i} = \begin{pmatrix}
	\sum_{t=1}^T H^{2*}_{i,t}x^2_{it,1} +  \frac{1}{2} \sum_{t=1}^T \sum_{s \neq t} H^{1*}_{i,t}x_{it,1} H^{1*}_{i,s} x_{is,1}\\
	\vdots \\
	\sum_{t=1}^T H^{2*}_{i,t}x^2_{it,q} +  \frac{1}{2} \sum_{t=1}^T \sum_{s \neq t} H^{1*}_{i,t}x_{it,q} H^{1*}_{i,s} x_{is,q} \\
	2 \sum_{t=1}^T H^{2*}_{i,t}x_{it,1} x_{it,2} +  \sum_{t=1}^T \sum_{s \neq t} H^{1*}_{i,t}x_{it,1} H^{1*}_{i,s} x_{is,2}\\
	\vdots \\
	2 \sum_{t=1}^T H^{2*}_{i,t}x_{it,1}x_{it,q} + \sum_{t=1}^T \sum_{s \neq t} H^{1*}_{i,t}x_{it,1} H^{1*}_{i,s} x_{is,q} \\
	2 \sum_{t=1}^T H^{2*}_{i,t}x_{it,2} x_{it,3} +  \sum_{t=1}^T \sum_{s \neq t} H^{1*}_{i,t}x_{it,2} H^{1*}_{i,s} x_{is,3}\\
	\vdots \\
	2 \sum_{t=1}^T H^{2*}_{i,t}x_{it,q-1}x_{it,q} + \sum_{t=1}^T \sum_{s \neq t} H^{1*}_{i,t}x_{it,q-1} H^{1*}_{i,s} x_{is,q}
	\end{pmatrix}
	\end{split},
\end{equation}
where $x_{it,k}$  denote the $k$-th component of the vector $x_{it} \in \R^q$.
Collect the relevant variables and define
\begin{equation}\label{t1}
t_n(\bs{\psi}_{\alpha},\alpha) := \begin{pmatrix}
n^{1/2} (\eta - \eta^*) \\
n^{1/2} \alpha ( 1- \alpha) v(\bs{\lambda})
\end{pmatrix}.
\end{equation}
Define the vector of outer product of $\lambda$ with itself as
\begin{equation}
% \label{eq:v}
\begin{split}
v(\bs{\lambda}  & =  (\lambda_{\mu}^2,\lambda_{\sigma}^2, \lambda_{\mu} \lambda_{\sigma^2}, \lambda_{\mu} \lambda_{\beta_1} , \ldots,\lambda_{\mu} \lambda_{\beta_q}, \lambda_{\sigma} \lambda_{\beta_1} , \ldots,\lambda_{\sigma} \lambda_{\beta_q},
  \lambda_{\beta_1}^2,\ldots,\lambda_{\beta_q}^2 ,
  \lambda_{\beta_1}^2,\ldots,\lambda_{\beta_q}^2, \\
  & \lambda_{\beta_1} \lambda_{\beta_2} ,
  \ldots,\lambda_{\beta_1} \lambda_{\beta_q},\lambda_{\beta_2} \lambda_{\beta_3},\ldots,\lambda_{\beta_2} \lambda_{\beta_q}, \ldots, \lambda_{\beta_{q-1}} \lambda_{\beta_{q}})^\top.
  \end{split}
\end{equation}
Define the normalized score
$S_n := n^{-1/2} \sum_{i=1}^N s_i$ and
the information matrix as $\bs{\mathcal{I}}_n := \frac{1}{n} \sum_{i=1}^N s_i s_i^\top,$.
%!!!!!!!!!!!!!!!!!!!!!!NOT SURE THIS IS GOOD
% By KS12 proposition A in appendix, the following are true:
% \begin{align*}
%   &\nabla_{\eta \lambda} l(\bs{w};\bs{\psi}_{\alpha},\alpha) = 0;
%   \E[\nabla_{\lambda_i,\lambda_j} l(\bs{w};\bs{\psi}^*_{\alpha},\alpha)] = 0 ;   \E[\nabla_{\lambda_i,\lambda_j,\lambda_k} l(\bs{w};\bs{\psi}^*_{\alpha},\alpha)] = O_p(n^{1/2}) ; \\
%   & \E[\nabla_{\eta \lambda_i \lambda_j} l(\bs{w};\bs{\psi}^*_{\alpha},\alpha) ] = - \E[\nabla_{ \eta}l(\bs{w};\bs{\psi}^*_{\alpha},\alpha) \nabla_{\lambda_i \lambda_j} l(\bs{w};\bs{\psi}^*_{\alpha},\alpha)], \\ & \E[\nabla_{\lambda_i \lambda_j \lambda_k \lambda_l} l(\bs{w};\bs{\psi}^*_{\alpha},\alpha) ] = - \E[\nabla_{\lambda_i \lambda_j} l(\bs{w};\bs{\psi}^*_{\alpha},\alpha) \nabla_{\lambda_k \lambda_l}l(\bs{w};\bs{\psi}^*_{\alpha},\alpha)  +  \\
%  & \nabla_{\lambda_i \lambda_k} l(\bs{w};\bs{\psi}^*_{\alpha},\alpha) \nabla_{\lambda_j \lambda_l} l(\bs{w};\bs{\psi}^*_{\alpha},\alpha) +  \nabla_{\lambda_i \lambda_l} l(\bs{w};\bs{\psi}^*_{\alpha},\alpha) \nabla_{\lambda_k \lambda_j} l(\bs{w};\bs{\psi}^*_{\alpha},\alpha)].
% \end{align*}

\subsection{Score function proof }

For each iteration $k$.
Given $\alpha_k^j,\mu_k^j,\sigma_k^j$, $\beta^j_k$.
First calculate square error $r_{i,k}^j = \sum_{t=1}^T \frac{1}{2}(\frac{y_{it} -\mu^j_k - x'_{it}\beta^j_k - z'_{it} \gamma_k}{\sigma^j_k})^2$, conditional on type-specific parameters.
For the finite mixture model, the likelihood for each $i$ is written
\begin{align*}
	f(\bs{w};\psi_0) & = \sum_{j=1}^j \alpha^j \left\{ \Pi_{t=1}^T \frac{1}{\sigma^j} \phi\left(\frac{ y_{it} -\mu^j - x'_{it}\beta^j - z'_{it} \gamma }{\sigma^j }\right)\right\} \\
	& = \sum_{j=1}^j \alpha^j \left\{ \Pi_{t=1}^T \frac{1}{\sqrt{2\pi}\sigma^j} \exp\{ \frac{- (y_{it} -\mu^j - x'_{it}\beta^j - z'_{it} \gamma)^2}{2 (\sigma^j)^2} \} \right\} \\
	& = \sum_{j=1}^j \alpha^j \left\{ \frac{1}{(\sqrt{2\pi}\sigma^j)^T} \exp\{ \frac{-\sum_{t=1}^T (y_{it} -\mu^j - x'_{it}\beta^j - z'_{it} \gamma)^2}{2 (\sigma^j)^2}\} \right\} \\
	& = \sum_{j=1}^j \alpha^j \left\{ \frac{1}{((\sqrt{2\pi} \sigma^j)^T} \exp\{-r_i^j\} \right\}.
\end{align*}
Call the weight matrix $W$ for Bayesian updating. In the $m \times N$ matrix, each element $ji$ represents the likelihood of firm $i$ belonging to type $j$.
$$
W' = \begin{pmatrix}
\frac{\alpha^1 f(\{\bs{W}_{1t}\}_{t=1}^T; \gamma,\theta^1)}{f(\{\bs{W}_{1t}\}_{t=1}^T; \gamma,\theta^1)} &\frac{\alpha^2 f(\{\bs{W}_{1t}\}_{t=1}^T; \gamma,\theta^2)}{f(\{\bs{W}_{1t}\}_{t=1}^T; \gamma,\theta^2)}& \ldots & \frac{\alpha^M f(\{\bs{W}_{1t}\}_{t=1}^T; \gamma,\theta^m)}{f(\{\bs{W}_{1t}\}_{t=1}^T; \gamma,\theta^m)} \\
\vdots & \vdots & \ddots & \vdots \\
\frac{\alpha^1 f(\{\bs{W}_{Nt}\}_{t=1}^T; \gamma,\theta^1)}{f(\{\bs{W}_{Nt}\}_{t=1}^T; \gamma,\theta^1)} &\frac{\alpha^2 f(\{\bs{W}_{Nt}\}_{t=1}^T; \gamma,\theta^2)}{f(\{\bs{W}_{Nt}\}_{t=1}^T; \gamma,\theta^2)}& \ldots & \frac{\alpha^M f(\{\bs{W}_{Nt}\}_{t=1}^T; \gamma,\theta^m)}{f(\{\bs{W}_{Nt}\}_{t=1}^T; \gamma,\theta^m)}
\end{pmatrix},
$$ where $w_{ij}^{(k)} = \frac{\alpha^{j(k)} f(\bs{w}; \gamma^{(k)},\theta^{j(k)})}{f(\bs{w}; \gamma^{(k)},\theta^{j(k)})}$ is the posterior probability of observation $i$ being type $j$ in $k$-th iteration .
Then update $\alpha^j, \mu^j, \sigma^j$ using $W$ at the end of each iteration, by the following formula.
Define $X_{it} = (X_{it,1},X_{it,2},\ldots,X_{it,q})'$,$\tilde{X}_{it} = (1,X_{it,1},X_{it,2},\ldots,X_{it,q})'$ and $Z_{it} = (Z_{it,1},Z_{it,2},\ldots,Z_{it,p})'$.
$\alpha^{j(k+1)} = \frac{1}{N} \sum_{i=1}^N w_{ij}^{(k)}$, is just the mean of each row from $W$. $\gamma$ is updated by  $$\gamma^{(k+1)} = (\sum_{i=1}^N \sum_{t=1}^T Z_{it} Z_{it}^T )^{-1} (\sum_{i=1}^{N}\sum_{t=1}^T Z_{it}(Y_i - \sum_{j=1}^{M_0} w_{ij}^{(k)} X_{it}^T\beta^{j(k)} - \mu^{j(k)})), $$
$\mu$ and $\beta$ is updated using
$$(\mu^{j(k+1)},(\beta^{j(k+1)})')' = (\sum_{i=1}^N \sum_{t=1}^T w_{ij}^{(k)} \tilde{X}_{it} \tilde{X}_{it}^T )^{-1} (\sum_{i=1}^{N}\sum_{t=1}^T \tilde{X}_{it}(Y_i - Z_{it}^T \gamma )) .$$

$\sigma^{j(k+1)}$ is the weighted average of residuals.
$$\sigma^{j(k+1),2} = \frac{1}{NT} \sum_{i=1}^N w_{it}^{(k)} \{ \sum_{i=1}^T  (y_{it} -\mu^{j(k)} - x'_{it}\beta^{j(k)} - z'_{it} \gamma^{(k)} )^2  \} .$$
